# Supplementary material for: Trustworthiness Evaluations of Search Results: The Impact of Rank and Misinformation
Source: arXiv:2309.11029 ancillary file (2023-09-20)
Supplement: Supplementary file 1 [file descriptive_statistics_copy.pdf]

## Descriptive statistics

For each experiment, we calculated descriptive statistics of the demographic attributes of each sample. We measured the following variables:

**Trust in the Search Engine.** We measured participants' general trust toward the search engine they saw by asking them to rate their agreement (1 = Strongly Disagree, 3 = Neither Agree nor Disagree, 5 = Strongly Agree) with six statements about the ability, benevolence, and integrity of the search engine from a formal model of organizational trust. We computed the average of these scores for each participant due to the high internal consistency (Cronbach's  $\alpha = 0.89$  for Google, Cronbach's  $\alpha = 0.88$  for DuckDuckGo).

**Vaccine Supportiveness.** We collected responses for six statements about the safety of vaccines for children to measure participants' general levels of support for childhood vaccination, which we also averaged to create a composite score for each participant (Cronbach's  $\alpha = 0.92$ ).

**Political Ideology.** Participants were asked to indicate their political alignment with a 5-point scale (1 = "Conservative", 5 = "Liberal").

**Age.** We asked participants to enter their age in years.

**Gender.** We asked participants to indicate their gender by selecting any of the following options: "Woman", "Man", "Nonbinary", and "Other."

Samples in the three experiments were similar in composition, as shown below:

|   | Summary_statistic      | Experiment 1 | Experiment 2 | Experiment 3 |
|---|------------------------|--------------|--------------|--------------|
| 1 | median_age             | 34           | 37           | 33           |
| 2 | mean_age               | 37.200       | 40.170       | 36.160       |
| 3 | sd_age                 | 13.420       | 14.620       | 12.870       |
| 4 | percent_men            | 50.401       | 49.098       | 48.750       |
| 5 | percent_women          | 47.896       | 48.497       | 48.833       |
| 6 | percent_NB             | 1.703        | 2.305        | 2.167        |
| 7 | median_liberalism      | 4            | 4            | 4            |
| 8 | median_vaccine_support | 4.333        | 4.167        | 4.167        |

|    |                               |        |        |        |
|----|-------------------------------|--------|--------|--------|
| 9  | mean_vaccine_support          | 4.030  | 4      | 3.980  |
| 10 | sd_vaccine_support            | 0.880  | 0.890  | 0.880  |
| 11 | median_trust_in_search_engine | 3.833  | 3.833  | 3.833  |
| 12 | mean_trust_in_search_engine   | 3.770  | 3.810  | 3.800  |
| 13 | sd_trust_in_search_engine     | 0.680  | 0.660  | 0.660  |
| 14 | percent_Google_users          | 87.375 | 87.976 | 89.500 |

Table S1: Descriptive statistics for each experiment.

### 6. Trustworthiness ratings

We calculated the average trustworthiness ratings of search results depending on their click status (clicked and non-clicked) and their information quality (accurate and misinformation), shown below. In each experiment, there were significant differences in trust levels toward accurate search results:

|   | study_id     | Click_status       | Info_quality         | n     | mean_trust | variance_trust | CI_trust     |
|---|--------------|--------------------|----------------------|-------|------------|----------------|--------------|
| 1 | Experiment 1 | Clicked result     | Accurate Information | 980   | 3.820      | 0.957          | (3.76, 3.88) |
| 2 | Experiment 1 | Clicked result     | Misinformation       | 18    | 2.940      | 1.467          | (2.38, 3.5)  |
| 3 | Experiment 1 | Non-clicked result | Accurate Information | 1,214 | 3.080      | 1.300          | (3.02, 3.14) |
| 4 | Experiment 1 | Non-clicked result | Misinformation       | 782   | 1.410      | 0.711          | (1.35, 1.47) |
| 1 | Experiment 2 | Clicked result     | Accurate Information | 315   | 3.150      | 1.019          | (3.04, 3.26) |

|   |              |                    |                      |     |       |       |               |
|---|--------------|--------------------|----------------------|-----|-------|-------|---------------|
| 2 | Experiment 2 | Clicked result     | Misinformation       | 9   | 2.670 | 1.750 | (1.81, 3.53)  |
| 3 | Experiment 2 | Non-clicked result | Accurate Information | 455 | 2.580 | 1.267 | (2.48, 2.68)  |
| 4 | Experiment 2 | Non-clicked result | Misinformation       | 219 | 1.640 | 1.158 | (1.5, 1.78)   |
| 1 | Experiment 3 | Clicked result     | Accurate Information | 440 | 2.900 | 1.145 | (2.8, 3)      |
| 2 | Experiment 3 | Clicked result     | Misinformation       | 3   | 2.330 | 5.333 | (-0.28, 4.94) |
| 3 | Experiment 3 | Non-clicked result | Accurate Information | 606 | 2.300 | 1.326 | (2.21, 2.39)  |
| 4 | Experiment 3 | Non-clicked result | Misinformation       | 151 | 1.560 | 1.048 | (1.4, 1.72)   |

Table S2: Average trustworthiness ratings for search results in each experiment.
