# Supplementary material for: Trustworthiness Evaluations of Search Results: The Impact of Rank and Misinformation
Source: arXiv:2309.11029 ancillary file (2023-09-20)
Supplement: Supplementary file 2 [file pretests_copy.pdf]

## **Pretests of stimuli**

Below, we detail the validation pretest procedures and results for each experiment. All participants recruited in the pretests were excluded from participating in any of the three main experiments.

### **B. 1. Misinformation for Experiments 1 & 2**

Our experiments involved manipulating whether one of the top three search results had misinformation; however, people often disagree over what information constitutes “misinformation,” especially in rapidly emerging situations such as Covid-19. To ensure that our manipulation was effective, we pretested five examples of misinformation results for each Covid-19 query. We recruited 30 participants from different political and socioeconomic backgrounds. As in the main experiment, we showed them pages of ten results for each query in a randomized order. Five of these results were examples that had misinformation, such as claiming that the Covid-19 vaccines cause cancer. The other five results had what we defined as “accurate information,” which were results from reputable medical sources that said the vaccines are safe. We asked participants to click on any results that they believed had false information. We used the three misinformation results that were selected most frequently for each query among those chosen by at least 80% of participants and used these in our main experiment. (Note: two of the misinformation results had a tie for one of the queries, but both came from the same source; to diversify the sources of misinformation, we used the fourth most frequently picked result in place of one of the tied ones). This pretest also confirmed that our accurate results were rarely chosen by participants as being false. See the “Stimuli” folder on the project’s

OSF repository ([https://osf.io/n2b3s/?view\\_only=0ae0c8d5d110493d933ab76a633fedd6](https://osf.io/n2b3s/?view_only=0ae0c8d5d110493d933ab76a633fedd6)) for the final search results we used in the main experiment.

## **B. 2. Uncertain Queries for Experiment 3**

Experiment 3 used three new Covid-19 queries whose answers were highly uncertain and unestablished among the medical community. We searched Google to find several examples of questions about Covid-19 that had a lack of consensus among medical sources (defined either as queries with medical sources saying that the answers were still unknown, or queries with multiple medical sources providing answers that were in opposition to each other). We then pretested these queries on a sample of participants from Prolific ( $n = 80$ ) to verify that participants would be aware of these queries' uncertainty. We showed the queries in randomized order and asked these participants to indicate their answers (options were “yes,” “no,” or “I don't know”). We also mixed in some questions that were more certain to give participants some questions they would feel confident of the answers to; we did this to prevent them from changing their answers to the uncertain questions in order to appear more knowledgeable. In addition, we asked participants to rate how personally relevant the questions were to them (measured with a 5-point Likert scale anchored at “extremely irrelevant” and “extremely relevant”), so that we could ensure the questions we used would still be interesting to participants during the main experiment.

We computed two uncertainty metrics for each query: the percentage of participants who selected “unsure,” and an ordinal value for how evenly split the answers were among the three options given (e.g., a query that had exactly 33% of respondents answering each option would have a value of 1). We compared the top queries for each of these metrics and found that the

ones that had the highest percentage of “I don’t know” responses were generally lower in relevance ratings than the queries that were the highest in dispersion, so we chose the top three queries with the highest dispersion values. The final selected queries used in Experiment 3 are shown in the “Stimuli” folder on the project’s OSF repository ([https://osf.io/n2b3s/?view\\_only=0ae0c8d5d110493d933ab76a633fedd6](https://osf.io/n2b3s/?view_only=0ae0c8d5d110493d933ab76a633fedd6)).

### **B. 3. Misinformation for Experiment 3**

Due to the lack of surefire answers to the new, uncertain queries used in Experiment 3, we created our own examples of misinformation results (containing generalized misinformation about the pandemic). We doctored five pieces of misinformation to look like the content of real search results, and we pretested them on a new group of Prolific participants ( $n = 80$ ). Similar to our pretest of the queries, we showed participants these search results’ misinformation mixed in randomized order with search results containing accurate information. We asked participants to rate the perceived accuracy of the content (measured using a 6-point Likert scale anchored at “definitely false” and “definitely true”), and the perceived likelihood of seeing it on a page of search results (measured using a 7-point Likert scale anchored at “very unlikely” and “very likely”). We added this second question to find examples that people recognized as false but also felt could plausibly appear in online searches, in order to make our experimental setup more realistic.

For each query, there were significant differences in average accuracy and realism ratings of the results with accurate information and misinformation, confirming that our examples were perceived to be misinformation. We then conducted pairwise t-tests of accuracy and realism ratings among the individual misinformation results for each query (with Bonferroni p value

adjustments). When there was a result excluding those that had significantly higher accuracy ratings than the others, we excluded it from consideration. (There were never any significant differences in realism ratings among these results). From the remaining results, we selected the three with the lowest median accuracy scores for each query. The final misinformation results had an overall average accuracy rating of 1.5 out of 6 scale points, and an overall average realism rating of 3.1 out of 7 scale points. These results are shown in the “Stimuli” folder on the project’s OSF repository ([https://osf.io/n2b3s/?view\\_only=0ae0c8d5d110493d933ab76a633fedd6](https://osf.io/n2b3s/?view_only=0ae0c8d5d110493d933ab76a633fedd6)).

### **Unfamiliar Sources for Experiments 2 and 3**

To compare whether people showed different search tendencies from Experiment 1 when they did not have prior knowledge about the search results’ sources, we obtained several source URLs from real Google search results that were uncommon (appearing on several pages after the first page of results and unrecognizable to the researchers). To validate our judgments and find the sources that were most unknown to participants on Prolific, we ran a pretest of these sources on a separate group of participants ( $n = 66$ ) from those recruited in our main experiments. We showed these participants a series of URLs in randomized order, including: 18 uncommon websites, 8 common websites, and 15 fake websites whose names we fabricated (our goal was to use real websites that were unknown, but we included the fake sites in case all of the real sites that we believed were unknown were actually widely recognized by participants. This scenario did not materialize, so we were able to discard the fake sites from consideration). For each, we asked participants to indicate whether they recognized the website (options were “Yes, I recognize this website” “No, I do not recognize this website,” and “I’m not sure if I recognize

this website”). We also asked participants to indicate whether they believed the website sounded real or fake (options were “This website sounds real,” “This website sounds fake,” or “I’m not sure if this website sounds real or fake”); we included this question to eliminate websites that were frequently rated as sounding fake, to support the realistic setup of our main experiments.

We started by summing the percentages of participants who answered that they did not recognize a site or were unsure if they recognized it (hereafter referred to as “unknownness”). This led us to discard an outlier that had the lowest unknownness score. We then consulted the answers to the question about whether each site sounded real or fake, and eliminated four more sites that had low percentages of participants who indicated that they sounded realistic. We were then left with 13 unknown sites, all of which had unknownness scores of at least 87.5%. These source URLs are shown in the “Stimuli” folder on the project’s OSF repository ([https://osf.io/n2b3s/?view\\_only=0ae0c8d5d110493d933ab76a633fedd6](https://osf.io/n2b3s/?view_only=0ae0c8d5d110493d933ab76a633fedd6)).
