# Supplementary material for: Trustworthiness Evaluations of Search Results: The Impact of Rank and Misinformation
Source: arXiv:2309.11029 ancillary file (2023-09-20)
Supplement: Supplementary file 3 [file stimuli_copy.pdf]

## Stimuli

**Queries.** Participants in Experiments 1 and 2 were randomly assigned to complete the survey for one of the following queries, shown in either a Google or DuckDuckGo search bar depending on the condition assignment:

1. “Are covid vaccines safe for children?”
2. “Can covid vaccines cause infertility later in life for children?”
3. “Can covid vaccines cause cancer in children?”

In Experiment 3, participants were randomly assigned to complete the survey for one of the following new queries that were pretested and found to be highly uncertain to participants (see the “Pretests” folder on the project’s OSF repository ([https://osf.io/n2b3s/?view\\_only=0ae0c8d5d110493d933ab76a633fedd6](https://osf.io/n2b3s/?view_only=0ae0c8d5d110493d933ab76a633fedd6) for details):

1. “Can animals transmit covid-19 to humans?”
2. “Is it recommended to wear two face masks to prevent covid-19 infection?”
3. “Is natural immunity from covid-19 more effective than immunity from the vaccine?”

**Search results.** We used Google to find real search results with accurate information and misinformation for the queries used in each experiment. The only exception to this was in Experiment 3, whose queries lacked clear misinformation on Google at the time of the experiment: as a result, we created our own examples of misinformation for each of these queries. In two separate pretests, we validated our misinformation results by asking participants to select results they believed to be misinformation from a list with a mixed list. One of these was randomly selected to be shown to each participant in the misinformation conditions at the corresponding rank and was surrounded by the first nine of the accurate results in a randomized order. Experiment 1 showed the results as they originally appeared on Google with their actual source URLs; we stripped these URLs from each result in Experiment 2 and instead assigned each text snippet to be paired with unfamiliar sources (see below). Experiment 3 used a new set of results for the new queries, with the same source-matching procedure as in Experiment 2. See Figure S1 - Figure S14 below for the exact results used.

The following are the search results as shown in Experiment 1 for each query; the same results were used in Experiment 2 with different sources:

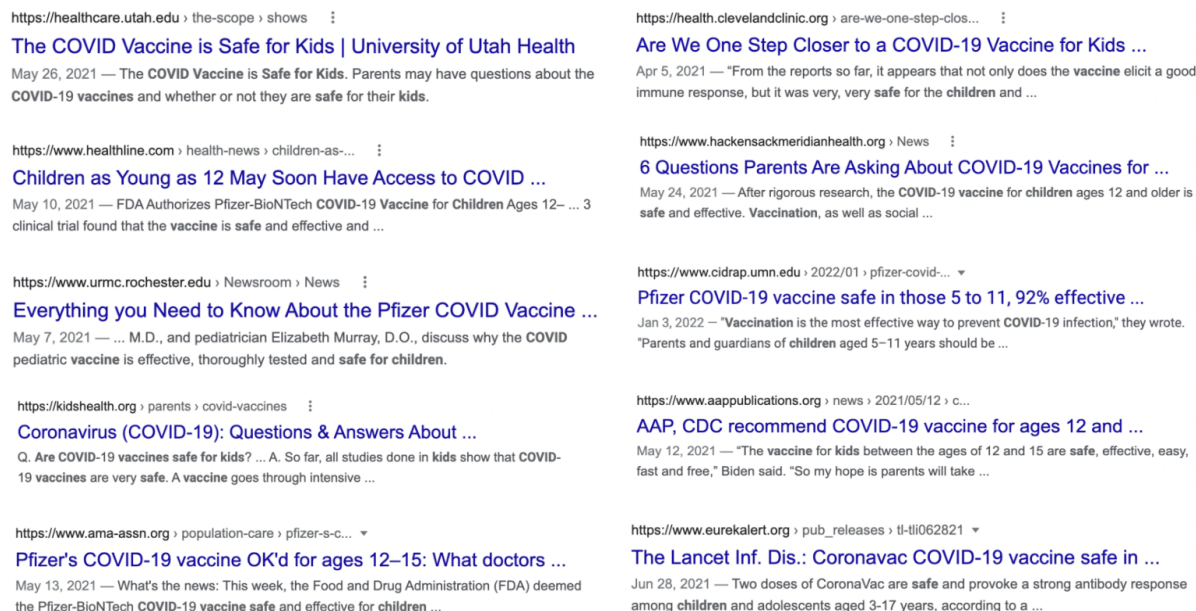

Figure S1: Accurate results for the query “Are covid vaccines safe for children?” in Experiment 1 and Experiment 2.

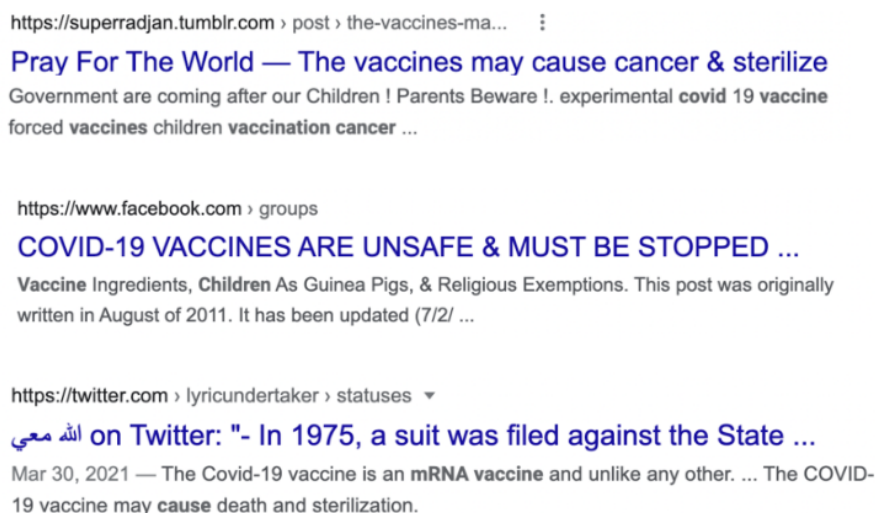

Figure S2: Misinformation results for the query “Are covid vaccines safe for children?” in Experiment 1 and Experiment 2.

<https://news.northwestern.edu/stories/2021/05/vac...>

**Worried your vaccinated pre-teen will become infertile? Don't be.**  
 May 11, 2021 — ... **COVID-19 vaccine** for adolescents, the next step will be to overcome ... To help fight vaccine hesitancy among teens, parents of teens, ... that the **COVID vaccine causes infertility**, which is gaining steam on social media.

<https://www.healthline.com/health-news/dont-let-mi...>

**COVID-19 Vaccines Cannot Affect Your Fertility - Healthline**  
 Jun 1, 2021 — Don't Let Misinformation About Fertility and COVID-19 Vaccines Stop Teens from ... The misconception that vaccines can cause infertility isn't new. ... "My advice for teens and parents concerned that the vaccine could impact ...

<https://www.muhealth.org/our-stories/does-covid-19...>

**Does the COVID-19 Vaccine Affect Fertility? Here's What the ...**  
 "While studies are ongoing, there is no data that the COVID-19 vaccines may cause infertility and no credible scientific theories for how the COVID-19 vaccine ...

<https://www.sciencedaily.com/releases/2022/01/>

**COVID-19 vaccines do not cause infertility, study finds**  
 Jan 20, 2022 — New findings indicate that COVID-19 vaccination does not impair fertility, but males who become infected by the coronavirus may experience ...

<https://news.llu.edu/health-wellness/does-covid-19-v...>

**Does the COVID-19 vaccination cause infertility? | LLUH News**  
 Jan 20, 2021 — According to Loma Linda University Health physicians, there is no evidence that the COVID-19 vaccines cause infertility. As people across the ...

<https://www.webmd.com/.../News>

**Why COVID Vaccines are Falsely Linked to Infertility - WebMD**  
 Jan 12, 2021 — There's no evidence that the new vaccines against COVID-19 cause infertility, yet that's a worry that's been cited by some health care workers ...

<https://www.henryford.com/blog/2021/04/fertility...>

**Here's Where That COVID-19 Vaccine Infertility Myth Came ...**  
 Apr 23, 2021 — "There is no evidence that shows getting one of the COVID-19 vaccines will cause infertility or even cause complications that would require ...

<https://www.sciencenews.org/article/covid-vaccine-i...>

**No, COVID-19 vaccines don't cause infertility | Science News**  
 Nov 11, 2021 — At the clinic, community health volunteers often are asked about the misinformation about the coronavirus vaccines and fertility. CFK Africa ...

<https://www.nebraskamed.com/COVID/you-asked-...>

**You asked, we answered: Can mRNA vaccines cause ...**  
 Dec 17, 2020 — The COVID-19 mRNA vaccines now have been in tens of thousands of people and infertility has not been a problem for men or women.

<https://www.verywellfamily.com/can-the-covid-19-va...>

**COVID-19 Vaccine Does Not Affect Male Fertility - Verywell ...**  
 SARS-CoV-2 RNA in Semen · No Change in Sperm After Vaccine · COVID-19 Infection and Male Fertility · How Does the mRNA Vaccine Work? · What Is the Vaccine Made Of?

Figure S3: Accurate results for the query “Can covid vaccines cause infertility later in life for children?” in Experiment 1 and Experiment 2.

<https://www.quora.com/How-risky-is-the-COVID-19-va...>

**How risky is the COVID-19 vaccination for people trying to ...**  
 VERY, VERY, VERY risky! Don't take it. There have been reports (in the Epoch Times) of 34 pregnant women experiencing spontaneous miscarriage or ...

<https://ar-ar.facebook.com/posts> [Translate this page](#)

**Loretta Lyn NY - Warnings of Infertility Come Directly With ...**  
 Dec 6, 2020 — Warnings of Infertility Come Directly With Pfizer Vaccine... ... Head of Pfizer Research: Covid Vaccine is Female Sterilization. The vaccine ...

<https://brandnewtube.com/watch/infertility-risks-of-...>

**Infertility Risks Of COVID-19 Injections, Spike Protein ...**  
 May 31, 2021 — Spike proteins, or what ever that may be, have been tested on rats to make them infertile. That crap is used in Covid Vaccines as well.

Figure S4: Misinformation results for the query “Can covid vaccines cause infertility later in life for children?” in Experiment 1 and Experiment 2.

<https://immunizebc.ca> › ask-us › questions › are-there-l... ⌵

### Are there long-term side effects caused by mRNA COVID-19 ...

Answer: The medical and scientific community is confident in the long-term safety of the mRNA COVID-19 vaccines. According to the USA ...

<https://www.sloankettering.edu> › coronavirus › what-yo... ⌵

### COVID-19 Vaccines Safety and Effectiveness | Memorial ...

COVID-19 Vaccine Safety and Effectiveness: Updated Information. English ... The vaccines do not cause cancer. They do not expose you to the virus that ...

<https://news.ship.edu> › 2021/05/11 › ariana-tomb-share... ⌵

### Ariana Tomb shares myths, facts and her own COVID vaccine ...

May 11, 2021 — The COVID vaccine is an RNA vaccine. RNA vaccines have in use for over 20 years to combat HIV, Zika, Rabies, and forms of cancer. They have been ...

<https://www.cancerresearch.org> › en-us › 30-facts ⌵

### Vaccines can help prevent cancers caused by viruses ...

Vaccines do not cause cancer — vaccines can actually help prevent cancers caused by viruses. Learn more about how vaccines use the immune system to fight ...

<https://onlinepublichealth.gwu.edu> › Resources ⌵

### Producing Prevention: How Vaccines Are Developed | Online ...

Jul 15, 2021 — Myth: COVID vaccines can cause false positive COVID test results. ... Fact: Vaccines are not connected to the development of autism, cancer, ...

<https://fullfact.org> › Health › Vaccines ⌵

### There's no evidence that any current vaccines cause cancer

Aug 29, 2019 — Vaccines go through a number of trial stages to check they don't have dangerous side effects.

<https://www.everydayhealth.com> › coronavirus › bigge... ⌵

### COVID-19 Vaccine Myths and Conspiracy Theories | Everyday ...

Jul 22, 2021 — No, COVID-19 vaccines do not infect you with the coronavirus or change your DNA. Read on for more vaccine misconceptions and conspiracy ...

<https://www.mskcc.org> › coronavirus › myths-about-co... ⌵

### Fact Check: 7 Persistent Myths about COVID-19 Vaccines ...

Myth: The mRNA vaccines change your DNA and could cause cancer. ... Truth: None of the vaccines interact with or alter your DNA in any way, and therefore cannot ...

<https://news.illu.edu> › health-wellness › expert-debunks... ⌵

### Expert debunks 5 COVID-19 vaccine misconceptions | LLUH ...

Mar 24, 2021 — Myth: Adenovirus technology is used in this vaccine, so it could cause cancer. Adenoviruses can cause a wide range of illnesses, such as the ...

<https://www.nature.com> › news explainer ⌵

### Should children get COVID vaccines? What the science says

Jul 20, 2021 — Thus far, the vaccines seem to be safe in adolescents, and some companies have moved on to carrying out clinical trials in children as young as ...

Figure S5: Accurate results for the query “Can covid vaccines cause cancer in children?” in Experiment 1 and Experiment 2.

<https://x.facebook.com> › CDC › photos ⌵

### CDC - If your child is Medicaid eligible, American Indian or ...

Jun 8, 2021 — Don't do it. Research. mRNA is in all child vaccines now and (HIV aborted fetal cells, since 1987) ... 2 H351 Suspected of causing cancer.

<https://twitter.com> › status ⌵ [Translate this page](#)

### Prasaanth Saran on Twitter: "The mRNA vaccine is coming to ...

Jan 9, 2021 — The mRNA vaccine is coming to the human race for the first time. This Genetic modification that causes the body to trigger cancer.

<https://www.reddit.com> › comments › what\_are\_some\_... ⌵

### What are some strange things or symptoms your patients have ...

For example, a recent patient blamed her jaundice on the covid vaccine she received 3 days ... Sounds to me like the COVID vaccine caused pancreatic cancer.

Figure S6: Misinformation results for the query “Can covid vaccines cause cancer in children?” in Experiment 1 and Experiment 2.

The following are Experiment 3’s search results for each query (these were randomly paired with the unfamiliar sources used in Experiment 2):

#### Pets don't transmit COVID-19

Dogs and cats in contact with infected humans have tested positive for COVID-19. However, there are no evidence to date that they can transmit COVID-19 to humans. Learn More.

#### Dog coronavirus jumps to humans, with a protein shift

... provide clues to how they transmit to humans from animals. A new canine coronavirus was first identified in two Malaysian human patients ...

#### People probably caught coronavirus from minks. That's a ...

After reports of infected dogs emerged from Hong Kong, they said there was no evidence animals could transmit the virus to humans.

#### Can pets transmit coronavirus to humans? No evidence so far ...

Experts say canine coronavirus is different from COVID-19, which is spreading now. And unlike COVID-19, the canine coronavirus has a vaccine ...

#### No evidence that animals can transmit the coronavirus to ...

No evidence that animals can transmit the coronavirus to humans · There is no current evidence of dogs playing a role in the spread of COVID-19.

#### Researchers identify first case of animal-to-human COVID ...

At first, researchers thought white-tailed deer were being infected by people, but new evidence shows it may also work the other way around.

#### Animals unlikely to spread Covid-19 to humans, but ...

There's no evidence that animals are playing a significant role in the spread of coronavirus to humans, but precautions can help keep people ...

#### A deer may have passed COVID-19 to a person, study suggests

She hopes “this will be the future of biosurveillance, where we will have to look across the spectrum of the animal kingdom—not just humans in ...

#### Pets are Blameless in Spread of COVID-19 Coronavirus

This is a case of human-to-animal transmission and means that dogs can carry low levels of the virus but don't become sick.

#### Your pets can catch coronavirus, but don't spread it

Cats and dogs don't tend to get very sick or transmit COVID-19, scientists say.

Figure S7: Accurate results for the query “Can animals transmit covid-19 to humans?” in Experiment 3.

#### The COVID VIRUS has never appeared in any animals

COVID is a HOAX!! it has never spread to animals so why do ppl put masks on their dogs?

#### Corona virus is fake disease and animals arent getting it

животные we all know covid is a fake disease ---animals have nothing to do with it...

#### URGENT: bats are biting humans and giving us corona virus

humans are getting sick with covid from bats biting them in texas!! spread the word to help others

Figure S8: Misinformation results for the query “Can animals transmit covid-19 to humans?” in Experiment 3.

#### Experts: Wearing 2 masks helps prevent COVID spread. But ...

A government study released on Wednesday, Feb. 10, 2021, finds that wearing two masks can better than one, in protecting against coronavirus ...

#### Covid-19: French doctors against wearing two masks

People in the US are being advised to 'double mask' to protect against ... Covid-19 group, told Le Parisien newspaper that there is "no ...

#### 1 Mask Is Good. Are 2 Masks Better? It Depends...

"Again, it's not a requirement to double mask. ... What's a good mask fit? ... Masks are critical for preventing the spread of COVID-19.

#### Wearing Two Masks Can Better Protect

You should wear two masks to avoid COVID — After the CDC recommended the use of two masks to protect from the With COVID-19, the higher the ...

#### Should You Double-Mask? It Depends

(If you do double up, the CDC recommends wearing one disposable mask underneath a cloth mask, but wearing two disposable masks is not advised.

#### Two masks could be one too many

Experts say double masking is a double-edged sword. ... Two masks could be one too many. Experts say double masking is a double-edged sword.

#### Wearing two masks only 4% more effective than wearing one ...

Japanese supercomputer simulations showed that wearing two masks gave ... better than one at reducing a person's exposure to the coronavirus.

#### Extra Layers Can Improve Face Masks' Effectiveness

The CDC does not recommend layering two disposable masks because "they are not designed to fit tightly, and wearing more than one will not ...

#### Why Two Face Masks Are Better Than One

With new, more contagious forms of COVID-19 spreading around the world, the Centers for Disease Control and Prevention (CDC) recommends that ...

#### Double masking amid COVID-19 not backed by research ...

A study concluding that wearing a disposable medical procedure mask under a reusable cloth face covering protects the wearer against ...

Figure S9: Accurate results for the query “Is it recommended to wear two face masks to prevent covid-19 infection?” in Experiment 3.

#### Covid is a hoax and masks dont do anything

the us government has fooled its' citizens by inventing a mysterious illness called covid.

#### according to "doctor" fauchi, masks are now a scam!

That's right, folks! Last night, "doctor" fauchi proclaimed that masks aren't working against covid and said we could stop using them...

#### Masks made of Tin foil now prevent alpha covid

in a recent news blast, we found out that tin foil can make us immune to the virus if crumpled over nose.

Figure S10: Misinformation results for the query “Is it recommended to wear two face masks to prevent covid-19 infection?” in Experiment 3.

#### COVID Vaccines and Infection Offer Similar Protection, Study ...

Getting vaccinated before or after getting infected with COVID-19 still provided a strong immune response. Natural infection and vaccination ...

#### COVID-19 vaccines more protective than 'natural' immunity

A new study concludes that a COVID-19 mRNA vaccine is around five times more effective at preventing hospitalization than a previous ...

#### COVID-19 infection may offer similar immunity as vaccination

Editor's note: On May 5, 2022, this story was corrected to clarify that no vaccinated people were involved in the study.

#### Why COVID-19 Vaccines Offer Better Protection Than Infection

Vaccination offers longer, stronger immunity, says virologist Sabra Klein.

#### Natural immunity stronger than vaccines alone in delta wave ...

Natural immunity was six times stronger during the delta wave than vaccination, according to a new report from the U.S. Centers for Disease ...

#### 'Bombshell' study finds natural immunity superior to vaccination

Researchers at Maccabi Healthcare and Tel Aviv University compared the outcomes of over 76,000 Israelis in three groups: the doubly vaccinated ( ...

#### Prior COVID infection more protective than vaccination during ...

People who had previously been infected with COVID-19 were better protected against the Delta variant than those who were vaccinated alone, ...

#### Previous Covid Prevents Delta Infection Better Than Pfizer Shot

People who recovered from a bout of Covid-19 during one of the earlier waves of the pandemic appear to have a lower risk of contracting the ...

#### Study shows vaccine immunity is stronger than natural immunity

The ZOE COVID Study, last month, found that vaccines offer greater protection against COVID-19 than natural antibodies.

#### COVID Vax 5 Times More Protective Than Natural Immunity

A new study shows that unvaccinated people who had a recent infection were five times more likely to be reinfected with the coronavirus ...

Figure S11: Accurate results for the query “Is natural immunity from covid-19 more effective than immunity from the vaccine?” in Experiment 3.

#### Don't get covid vaccines, they don't provide any imunity

join the anti-vax league and resist government control over our bodies!!медицинский.

#### COvid is a mild cold & immunity doesn't matter

Don't waste your time worrying about COVID it doesnt hurt your health

#### Covid vaccines have expired ingredients; they don't work now

Celery powder is used in the vaccines!! The ones made in December are now expired. So they are not providing actual immunity to covid now.

Figure S12: Misinformation results for the query “Is natural immunity from covid-19 more effective than immunity from the vaccine?” in Experiment 3.

**Unfamiliar sources:** In Experiments 2 and 3, we used the text portion of search results and randomly assigned each to have one of thirteen possible source URLs between subjects (this meant that three of the URLs were not shown for each participant). The following sources were found in a pretest to be unrecognizable to participants (see the “Pretests” folder on the project’s

OSF repository ([https://osf.io/n2b3s/?view\\_only=0ae0c8d5d110493d933ab76a633fedd6](https://osf.io/n2b3s/?view_only=0ae0c8d5d110493d933ab76a633fedd6)) for details):

<https://bannerhealth.com>, <https://castleconnolly.com>, <https://conehealth.com>, <https://grmedcenter.com>, <https://marrketnation.com>, <https://clinic.meijer.com>, <https://occovid19.ochealthinfo.com>, <https://parkview.com>, <https://samc.com>, <https://sbcovid19.com>, <https://smh.com>, <https://ssmhealth.com>, and <https://tipcobra.com>.

**Decoy Queries:** Participants in each experiment completed the same task for two decoy queries, “Is it safe to use cruise control in the rain?” and “Is a vegan diet safe for dogs?” We showed ten accurate results to everyone for these queries (shown below in Figure S13 and Figure S14) and did not analyze their data.

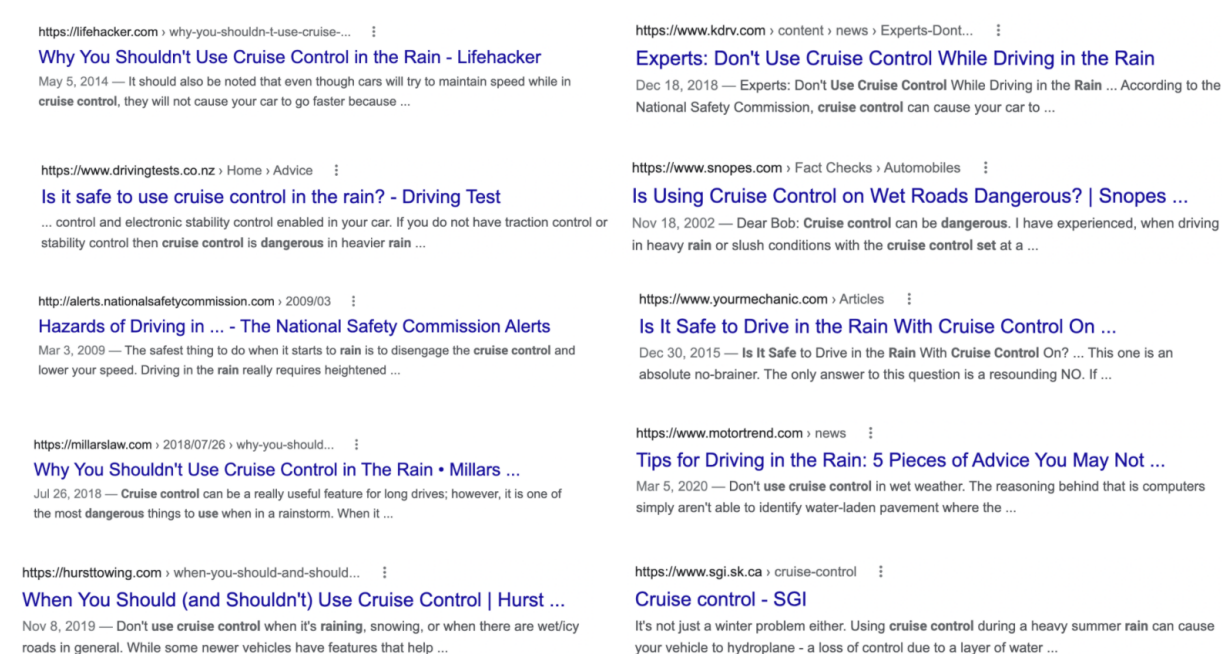

Figure S13: Accurate results shown in a random order in a single list for the decoy query “Is it safe to use cruise control in the rain?”

<https://www.hillspet.com> › ... › Nutrition & Feeding

### Can Dogs Be Vegan? | Hill's Pet

Apr 17, 2018 — The short answer is that yes, technically speaking, **dogs** can survive and even do well on a **vegan** or **vegetarian** regimen, says Cummings ...

<https://www.caninejournal.com> › vegan-dog-food

### A Comprehensive Guide To Vegan Dog Food ...

Oct 30, 2020 — Can **dogs** be vegan? While **dogs** prefer meat and animal products, many experts say it's possible to feed your **dog** a **vegan diet** — as long as you ...

<https://tractive.com> › can-feed-dogs-vegan-dog-food

### Vegan dog food: Pros & Cons for your dog's health | Tractive

May 19, 2021 — **Vegan dog** food is **safe**, as long as it contains enough nutrients for your **dog**. **Dog** parents need to be aware that conventional **dog** food also ...

<https://www.plantbased.dog>

### Plant-Based Dog Food

DOGS CAN THRIVE ON A HEALTHY PLANT-BASED DIET ... Find responses to common questions about **plant-based diets** for **dogs** with the FAQ explorer ...

<https://www.livekindly.co> › Lifestyle › Home & Living

### Is a Vegan Diet Safe for Cats? What Every Pet Lover Needs to ...

**Dogs** are omnivorous and can be fed a **vegan diet**, as long as it is **healthy** and **balanced**. As many cat owners will be aware, domesticated cats still have ...

<https://www.thesprucepets.com> › raising-your-dog-vega...

### Raising Your Dog Vegan - The Spruce Pets

Jun 22, 2020 — While we know that most **dogs** thrive on diets consisting of animal proteins, it is still possible to keep your **dog** **healthy** on a **vegan diet**. · One of the ...

<https://www.tomandsawyer.com> › Pet Health

### Can Dogs & Cats Eat Vegan? | Tom&Sawyer

It appears that **dogs** can, in many cases, be **safely** fed a **vegetarian diet**. Every individual **dog** reacts differently to a **vegetarian diet**, so they should be monitored ...

<https://www.germanshepherdrescue.co.uk> › Vegan-Diet...

### Healthy Vegan Diet For Dogs - German Shepherd Rescue

New Research Suggests **Dogs** Can Thrive on a **Plant-Based Diet**. Dogg Canine Nutrition Company, based in British Columbia, just completed the world's first-ever ...

<https://www.petsradar.com> › advice › can-a-dog-be-veg...

### Can a dog be vegan? We asked a vet... | PetsRadar

Mar 19, 2021 — That means that, theoretically, a **dog** can eat a **plant-based diet** and gain the right amino acids either from the plants, or from manufacturing their ...

<https://www.quora.com> › Is-it-possible-for-a-dog-to-stay-...

### Is it possible for a dog to stay healthy on a vegan diet? - Quora

Yes, **dogs** can be **healthy** on a **vegan diet** if the **dog** is willing to eat that way and the diet is nutritious enough. Just like people, they would need a variety of foods to ...

Figure S14: Accurate results shown in a random order in a single list for the decoy query “Is a vegan diet safe for dogs?”
